# Supplementary material for: Heavy-traffic Delay Optimality in Pull-based Load Balancing Systems: Necessary and Sufficient Conditions
Source: arXiv:1808.06911 source file (2018-08-21)
Supplement: Supplementary file 1 [file appendix.tex]

% !TEX root = ./sig2018_winter.tex
% \section{Appendix}
\appendix
\section{Proof of Lemma \ref{claim_1}}
\label{sec:proof_of_claim_1}
\begin{proof}

  Let us consider the Lyapunov function $V_1(\Q(t)) \triangleq \norm{\Q(t)}_1^2$, and the corresponding conditional mean drift is given by 
  \begin{align}
  \label{eq:heavy}
    &\ex{V_1(\Q(t+1)) - V_1(\Q(t)) \mid \Q(t) = \Q}\nonumber\\
    = & \ex{ \norm{\Q(t+1)}_1^2 - \norm{\Q(t)}_1^2 \mid \Q(t) = \Q    }\nonumber\\
    % = & \ex{\left(\norm{\Q(t)}_1+\norm{\A(t)}_1-\norm{\s(t)}_1 + \norm{\UU(t)}_1 \right)^2  \mid \Q(t) = \Q    }\nonumber\\
    % & - \ex{\norm{\Q(t)}_1^2 \mid \Q(t) = \Q   }\nonumber\\
        = & \mathbb{E}\left[ 2\norm{\Q{}}_1\left( \norm{\A}_1 - \norm{\s}_1\right) + \left( \norm{\A}_1-\norm{\s}_1\right)^2\right.\nonumber\\
         & +\left.{} 2\left(\norm{\Q}_1 +\norm{\A}_1 - \norm{\s}_1 \right) \norm{\UU}_1 + \norm{\UU}_1^2 \vphantom{\left( \norm{\A}_1-\norm{\s}_1\right)^2}      \mid \Q(t) = \Q   \right]\nonumber\\
        = & \mathbb{E}\left[ 2\norm{\Q}_1\left( \norm{\A}_1 - \norm{\s}_1\right) + \left( \norm{\A}_1-\norm{\s}_1\right)^2\right.\nonumber\\
         & +\left.{} 2\norm{\Q(t+1)}_1 \norm{\UU}_1 - \norm{\UU}_1^2 \vphantom{\left( \norm{\A}_1-\norm{\s}_1\right)^2}      \mid \Q(t) = \Q   \right].
  \end{align}
  By the definition of throughput optimality in this paper, we have $\ex{V_1(\overline{\Q})}$ is finite. Therefore, the mean drift of $V_1(.)$ is zero in steady-state. Taking expectation of both sides of Eq. \eqref{eq:heavy} with respect to the steady-state distribution $\overline{\Q}^{(\epsilon)}$, yields
  \begin{equation*}
  % \label{eq:sum_queuelength_equation}
    \epsilon \ex{\sum_{n=1}^{N}\overline{Q}_n^{(\epsilon)}} = \frac{\zeta^{(\epsilon)}}{2} + \ex{\big\lVert\overline{\Q}^{(\epsilon)}(t+1)\big\rVert_1 \big\lVert\overline{\UU}^{(\epsilon)} (t)\big\rVert_1} - \frac{1}{2}\ex{\big\lVert\overline{\UU}^{(\epsilon)}\big\rVert_1^2}
  \end{equation*}
  where $\zeta^{(\epsilon)} = (\sigma_\Sigma^{(\epsilon)})^2 + \nu_\Sigma^2 + \epsilon^2$. Then by utilizing the property of unused service shown in Lemma \ref{lem:unused_service}, we have 
  \begin{equation*}
    \frac{\zeta^{(\epsilon)}}{2} + {\mathcal{T}}^{(\epsilon)} - \frac{1}{2}c_1\epsilon \le \epsilon \ex{\sum_{n=1}^{N}\overline{Q}_n^{(\epsilon)}} \le \frac{\zeta^{(\epsilon)}}{2} + {\mathcal{T}}^{(\epsilon)},
  \end{equation*}
  in which ${\mathcal{T}}^{(\epsilon)} = \ex{\big\lVert\overline{\Q}^{(\epsilon)}(t+1)\big\rVert_1 \norm{\overline{\UU}^{(\epsilon)} (t)}_1}$. Since $\zeta^{(\epsilon)}$ converges to $\zeta$, from the inequality above and the definition of heavy-traffic delay optimality, we can easily see that the sufficient and necessary condition is $\lim_{\epsilon \downarrow 0} {\mathcal{T}}^{(\epsilon)} = 0$, which completes the proof of Lemma \ref{claim_1}. 
\end{proof}

\section{Proof of Lemma \ref{lemma:fluid model}}
\label{appendex:proof_fluid_model}
\begin{proof}
  (a) To show Eqs. \eqref{eq:sigma} and \eqref{eq:s} hold,  we can directly apply FSLLN (functional strong law of large numbers) to obtain that $\frac{1}{x_{n_k}}{\mathcal{A} }_{\Sigma}^{(x_{n_k})}(x_{n_k} t) \to \lambda t$ and $\frac{1}{x_{n_k}}{\mathcal{S} }_{i}^{(x_{n_k})}(x_{n_k} t) \to \mu_i t$, u.o.c, and each limiting function is Lipschitz continuous. 

  (b) For Eqs. \eqref{eq:g} and \eqref{eq:b}, for any given $0 \le t_1  \le t_2$, we have 
  \begin{equation}
  \label{eq:delta_g}
    0 \le \frac{1}{x_{n_k}} \left[ {\mathcal{G} }_{i}^{(x_{n_k})}(x_{n_k} t_2) - {\mathcal{G} }_{i}^{(x_{n_k})}(x_{n_k} t_1) \right] \le (t_2 - t_1).
  \end{equation}
  Therefore, the sequence of functions $\{\frac{1}{x_{n_k}}{\mathcal{G} }_{i}^{(x_{n_k})}(x_{n_k} t) \}$ is uniformly bounded and uniformly equicontinuous. As a result, by the Arzela-Ascoli theorem, there must exist a subsequence along which Eq. \eqref{eq:g} hold. In addition, Eq. \eqref{eq:delta_g} also implies that each limiting function $g_i$ is Lipschitz continuous. Same argument can be used to show Eq. \eqref{eq:b} hold and each limiting function $b_i$ is Lipschitz continuous.

  (c) For Eq. \eqref{eq:qq}, since the sequence $\{\frac{1}{x_n}Q_i^{x_n}(0)\}$ is upper bounded by 1 as a result of Eq. \eqref{eq:norm}, we have that there is a subsequence such that $\frac{1}{x_{n_k}}{Q}_i^{(x_{n_k})}(0) \to q_i(0)$. Hence, the convergence of Eq. \eqref{eq:qq} follows directly from Eq. \eqref{eq:q_dynamic}, and each limiting function $q_i$ is Lipschitz continuous.

  (d) To show that Eqs. \eqref{eq:ai} and \eqref{eq:di} hold, we utilize the fact that the arrival and departure process are bounded. Take the arrival process for example, we have 
  \begin{equation*}
  \label{eq:delta_ai}
    0 \le \frac{1}{x_{n_k}} \left[ {\mathcal{A} }_{i}^{(x_{n_k})}(x_{n_k} t_2) - {\mathcal{A} }_{i}^{(x_{n_k})}(x_{n_k} t_1) \right] \le A_{\max}(t_2 - t_1),
  \end{equation*}
  where $A_{\max}$ is the maximum number of exogenous arrivals at each time-slot. For each server $i$, we also have
  \begin{equation*}
  \label{eq:delta_di}
    0 \le \frac{1}{x_{n_k}} \left[ {\mathcal{D} }_{i}^{(x_{n_k})}(x_{n_k} t_2) - {\mathcal{D} }_{i}^{(x_{n_k})}(x_{n_k} t_1) \right] \le S_{\max}(t_2 - t_1),
  \end{equation*}
  where $S_{\max}$ is the maximum number of offered service at each time-slot. As a result, with the similar argument as in Eq. \eqref{eq:delta_g}, we can easily show Eqs. \eqref{eq:ai} and \eqref{eq:di} hold, and each limiting function is Lipschitz continuous. 
  % The other method doesn't rely on the fact of bounded arrivals and service, it is based on Theorem 5.3 in \cite{chen2013fundamentals}, which is repeated  in the next Theorem \ref{thm:random-time change}. We defer the second method to the following Lemma \ref{lemma:fluid limit}, which gives equations that each limiting function should satisfy.
\end{proof}

\section{Proof of Lemma \ref{lemma:fluid limit}}
\label{appendex:proof_fluid_limit}
In the proof, we will utilize the random time-change theorem in Chapter 5 of \cite{chen2013fundamentals}, which is presented below for easy reference.

\begin{theorem}[Random Time-Change Theorem]
\label{thm:random-time change}
Let $\{ X_n, n \ge 1\}$ and $\{ Y_n, n \ge 1\}$ be two sequences in ${D}^J$ (i.e., the space of $J$-dimensional real-valued functions on $[0,\infty)$ that are right-continuous and with left limits.). Assume that $Y_n$ is nondecreasing with $Y_n(0) = 0$. If as $n \to \infty$, $(X_n,Y_n)$ converges uniformly on compact sets to $(X,Y)$ with $X$ and $Y$ in ${C}^J$ (i.e., the space of $J$-dimensional real-valued continuous functions on $[0,\infty)$), then $X_n(Y_n)$ converges uniformly on compact sets to $X(Y)$, where $X_n(Y_n) = X_n \circ Y_n = \{X_n(Y_n(t)), t \ge 0 \}$ and  $X(Y) = X \circ Y = \{X(Y(t)), t \ge 0 \}$.
\end{theorem}

Now, we present the proof of Lemma \ref{lemma:fluid limit}.
\begin{proof}
  (a) Eqs. \eqref{eq:fluid_a_all} and \eqref{eq:fluid_s} directly follows from FSLLN under our assumptions for the exogenous arrival process and each service process.

  (b) Eq. \eqref{eq:fluid_q} follows from the definition of the queue length dynamic. Eq. \eqref{eq:sum_g} follows from the definition directly.

  (c) Eqs. \eqref{eq:fluid_ai} and \eqref{eq:fluid_di} are the results of Theorem \ref{thm:random-time change}. More specifically, let $X_n = \frac{1}{x_{n_k}}{\mathcal{A} }_{\Sigma}^{(x_{n_k})}(x_{n_k} t)$ and $Y_n = \frac{1}{x_{n_k}}{\mathcal{G} }_{i}^{(x_{n_k})}(x_{n_k} t)$ and we have $(X_n,Y_n) \to (\lambda t, g_i(t))$ uniformly on compact set, and $Y_n$ is nondecreasing with $Y_n(0) = 0$. Thus by Theorem \ref{thm:random-time change}, we have $X_n(Y_n(t)) = \frac{1}{x_{n_k}}{\mathcal{A} }_i^{(x_{n_k})}(x_{n_k} t) \to X(Y(t)) = \lambda g_i(t) = a_i(t)$ uniformly on compact sets. Similar argument can be used to show Eq. \eqref{eq:fluid_di} hold.

  (d) Note that $t$ is the regular time in Eq. \eqref{eq:derivative}, and hence $q_i^{\prime}(t)$ is well defined and exists. Therefore, the left-derivative $q_i^{\prime}(t-)$ should be equal to the right-derivative $q_i^{\prime}(t+)$. By the non-negativity of $q_i(t)$, if $q_i(t) = 0$, then we must have $q_i^{\prime}(t-) \le 0$ and $q_i^{\prime}(t+) \ge 0$, which results in $q_i^{\prime}(t) = 0$.
    For the case $q_i(t) > 0$, we need to show $d_i^{\prime}(t) = \mu_i$. It suffices to consider the right-derivative as it is equal to the derivative at a regular time $t$. Suppose $q_i(t) > 0$, then by the continuity of $q_i(t)$, there exists a $\delta > 0$, such that $a = \min_{t_s\in[t,t+\delta]}q(t_s) > 0$. Therefore, for sufficient large $x_{n_k}$, we have
    \begin{equation}
      \frac{1}{x_{n_k}}{Q}_i^{(x_{n_k})}(x_{n_k} t_s) \ge \frac{a}{2}, \text{for any  } t_s\in[t,t+\delta] \text{ and } \frac{a}{2}x_{n_k} \ge 1,
    \end{equation}
    which implies that ${Q}_i^{(x_{n_k})}(x_{n_k} t) \ge 1$ for any $t_s \in [t,t+\delta]$. Therefore, we have
    \begin{align*}
      &\frac{1}{x_{n_k}}{\mathcal{D} }_i^{(x_{n_k})}(x_{n_k} t_s) - \frac{1}{x_{n_k}}{\mathcal{D} }_i^{(x_{n_k})}(x_{n_k} t) \\
      = &\frac{1}{x_{n_k}}{\mathcal{S} }_i^{(x_{n_k})}(x_{n_k} t_s) - \frac{1}{x_{n_k}}{\mathcal{S} }_i^{(x_{n_k})}(x_{n_k} t).
    \end{align*}
    Then, according to the definition of derivative, we have 
    \begin{equation}
    \begin{split}
      d_i^{\prime}(t) &= \lim_{t_s\to t}\lim_{x_{n_k} \to \infty} \frac{1}{x_{n_k}}\frac{{\mathcal{D} }_i^{(x_{n_k})}(x_{n_k} t_s) - {\mathcal{D} }_i^{(x_{n_k})}(x_{n_k} t)}{t_s - t}\\
      & = \lim_{t_s\to t}\lim_{x_{n_k} \to \infty} \frac{1}{x_{n_k}}\frac{{\mathcal{S} }_i^{(x_{n_k})}(x_{n_k} t_s) - {\mathcal{S} }_i^{(x_{n_k})}(x_{n_k} t)}{t_s - t}\\
      & = \mu_i
    \end{split}
    \end{equation}
    As a result, Eq. \eqref{eq:derivative} is true for any regular time $t$.
\end{proof}

\section{Proof of Claim \ref{claim_2}}
\label{sec:proof_of_Claim_2}
\begin{proof}
Since $q_{\sigma_t(m+1)}(t) > 0$, $q_{\sigma_t(m)}(t) = 0$ and both functions are continuous, we can choose a $\tau$ such that $a/b > 4/\alpha$ where $a = \min_{t_s\in[t-\tau,t+\tau]}q_{\sigma_t(m+1)}(t_s)$ and $b = \max_{t_s\in[t-\tau,t+\tau]}q_{\sigma_t(m)}(t_s)$. By the u.o.c convergence, for sufficient large $x_{n_k}$, we have for any $t_s\in[t-\tau,t+\tau]$
  \begin{equation}
      \frac{1}{x_{n_k}}{Q}_{\sigma_t(m+1)}^{(x_{n_k})}(x_{n_k} t_s) \ge \frac{a}{2} \text{ and } \frac{1}{x_{n_k}}{Q}_{\sigma_t(m)}^{(x_{n_k})}(x_{n_k} t_s) \le 2b,
    \end{equation}
    which implies that ${{Q}_{\sigma_t(m+1)}^{(x_{n_k})}(x_{n_k} t_s)}\big/{{Q}_{\sigma_t(m)}^{(x_{n_k})}(x_{n_k} t_s)} > 1/\alpha$, for any $t_s\in [t-\tau,t+\tau]$. This indicates that in the interval $[(t-\tau)x_{n_k} + 1,(t+\tau)x_{n_k}-1]$, the queue-length state is outside the cone $\mathcal{K}_\alpha$. In this case, according to the conditions for the load balancing policy in Theorem \ref{thm:theorem_2}, we have 
    \begin{align*}
      \sum_{n=m+1}^N & \left(\frac{1}{x_{n_k}}{\mathcal{G} }_{\sigma_t(n)}^{(x_{n_k})}(x_{n_k} (t+\frac{\tau}{2})) - \frac{1}{x_{n_k}}{\mathcal{G} }_{\sigma_t(n)}^{(x_{n_k})}(x_{n_k} (t-\frac{\tau}{2}))\right)\\
      & = \tau \sum_{n=m+1}^N \left(\Delta_n(t) + \frac{\mu_{\sigma_t(n)}}{\mu_{\Sigma}}\right).
    \end{align*}
    By letting $x_{n_k} \to \infty$ and from Eq.\eqref{eq:g}, we have 
    \begin{equation*}
      \sum_{n=m+1}^N  \left(g_{\sigma_t(n)}(t+\frac{\tau}{2}) - g_{\sigma_t(n)}(t+\frac{\tau}{2})\right) = \tau \sum_{n=m+1}^N \left(\Delta_n(t) + \frac{\mu_{\sigma_t(n)}}{\mu_{\Sigma}}\right),
    \end{equation*}
    which directly implies the required result of Claim \ref{claim_2}.
\end{proof}

\section{Proof of Claim \ref{claim_3}}
\label{sec:proof_of_Claim_3}
\begin{proof}
  First, we have the following bound 
  \begin{align}
  \label{eq:root_bound}
    &\ex{\Delta V_\perp(\Q) \mid \Q(t) = \Q }\nonumber \\
    \le &\frac{1}{2\norm{\Qc}}\ex{\Delta W(\Q)  - \Delta W_{\parallel}(\Q)\mid \Q(t) = \Q}.
  \end{align}
  Similar to Lemma 7 in \cite{eryilmaz2012asymptotically}, this bound directly follows from the concavity of root function and  Pythagorean theorem. Next, we will bound each term in Eq. \eqref{eq:root_bound}, respectively. To begin with, we have an upper bound for the first term as follows.
  \begin{align}
  \label{eq:root_bound_W}
    &\ex{\Delta W(\Q) \mid \Q(t) =  \Q}\nonumber\\
    = &\ex{\norm{\Q(t) + \A(t)-\s(t) +\UU(t)}^2- \norm{\Q(t)}^2 \mid \Q}\nonumber\\
    \lep{a} &\ex{\norm{\Q(t) + \A(t)-\s(t)}^2- \norm{\Q(t)}^2 \mid \Q}\nonumber\\
    = &\ex{2\inner{\Q(t)}{\A(t)-\s(t)} + \norm{\A(t)-\s(t)}^2 \mid \Q}\nonumber\\
    \lep{b}& \ex{2\inner{\Q(t)}{\A(t)-\s(t)}\mid \Q }+ L
  \end{align}
  where (a) holds as $[\max(a,0)]^2 \le a^2 $ for any $a\in \mathbb{R}$; in (b), $L \triangleq N\max(A_{\max},S_{\max})^2$, which follows from the assumptions that  $A_\Sigma(t) \le A_{\max}$ and $S_n(t) \le S_{\max}$ for all $t \ge 0$ and all $ 1\le n \le N$, and the fact that they are both independent of the queue lengths. 

  We now turn to provide a lower bound on the second term in Eq. \eqref{eq:root_bound} as follows.
  \begin{align}
  \label{eq:root_bound_Wp}
        &\ex{\Delta W_\parallel(\Q) \mid \Q(t) =  \Q}\nonumber\\ 
        = & \ex{ 2\inner{\Qp(t)}{\Qp(t+1) - \Qp(t)} + \norm{\Qp(t+1) - \Qp(t)}^2\mid \Q}\nonumber\\
        \ge & \ex{2\inner{\Qp(t)}{\Qp(t+1) - \Qp(t)} \mid \Q}\nonumber\\
        = &2 \ex{\inner{\Qp(t)}{\Q(t+1) -\Q(t)} - 2\inner{\Qp(t)}{\Qc(t+1) - \Qc(t)} \mid \Q}\nonumber\\
        \gep{a} & \ex{2 \inner{\Qp(t)}{\Q(t+1) -\Q(t)}\mid \Q } \nonumber\\
        \gep{b} & \ex{2 \inner{\Qp(t)}{\A(t)-\s(t)} \mid \Q}
  \end{align}
  where (a) holds because $\inner{\Qp(t)}{\Qc(t)} = 0$ and $\inner{\Qc(t+1)}{\Qp(t)} \le 0$, since $\Qp(t) \in \mathcal{K}_{\alpha}$ and $\Qc(t+1)\in \mathcal{K}_{\alpha}^{\circ}$; (b) follows from the fact that all the components of $\Qp(t)$ and $\UU(t)$ are nonnegative.
    Thus, substituting Eqs. \eqref{eq:root_bound_W} and \eqref{eq:root_bound_Wp} into Eq. \eqref{eq:root_bound}, yields the bound in Claim \ref{claim_3}.
\end{proof}

\section{Proof of Claim \ref{claim_4}}
\label{sec:proof_of_Claim_4}
\begin{proof}
  This claim can be proved by contradiction. Suppose $m \in \mathcal{I}$ but $m+1 \notin \mathcal{I}$, then by the definition of $\mathcal{I}$, we have $w_{m} >0$ and $w_{m+1} = 0$. From the definition of $\mathbf{b}^{(i)}$ and the fact that $\widehat{\Q}_{\parallel}(t) = \sum_{i \in \mathcal{I}} w_i\mathbf{b}^{(i)}$, we have 
  \begin{align*}
    \widehat{Q}_{\parallel m}(t) - \widehat{Q}_{\parallel m+1}(t) = w_m(1-\alpha) > 0,
  \end{align*}
  which implies that 
  \begin{align}
  \label{eq:qc_larger}
    \widehat{Q}_{\perp m}(t) < \widehat{Q}_{\perp m+1}(t),
  \end{align}
  since $\widehat{Q}_m(t) \le \widehat{Q}_{m+1}(t)$. Then, it follows that 
  \begin{align*}
    \inner{\widehat{\Q}_{\perp}(t)}{\mathbf{b}^{(m+1)}} &= \alpha \sum_{n=1}^N \widehat{\Q}_{\perp n}(t) + (1-\alpha)\widehat{Q}_{\perp m+1}(t)\\
    & \gp{a} \alpha \sum_{n=1}^N \widehat{\Q}_{\perp n}(t) + (1-\alpha)\widehat{Q}_{\perp m}(t)\\
    & = \inner{\widehat{\Q}_{\perp}(t)}{\mathbf{b}^{(m)}}\\
    & \ep{b} 0
  \end{align*}
  where (a) follows from Eq. \eqref{eq:qc_larger}; and (b) comes from Eq. \eqref{eq:i_in_I}. However, by Eq. \eqref{eq:all_i}, we must have $\inner{\widehat{\Q}_{\perp}(t)}{\mathbf{b}^{(m+1)}} \le 0$. Hence, Claim~\ref{claim_4} is true.
\end{proof}

\section{Proof of Proposition \ref{prop:prop_3}}
\label{sec:proof_prop_3}
\begin{proof}
  It follows from Lemma~\ref{claim_1} and the proof of Theorem~\ref{thm:theorem_1} that the key for heavy-traffic delay optimality is the term $\mathcal{T}^{(\epsilon)}$. Instead of using Cauchy-Schwartz inequality, we apply H\"older inequality in Eq. \eqref{eq:upper_T} to obtain a tighter bound of $\mathcal{T}^{(\epsilon)}$ as follows. 
  \begin{align}
  \label{eq:upper_T_general}
    \mathcal{T}^{(\epsilon)} & \le \ex{\inner{\overline{\UU}}{-N_1\overline{\Q}^+_{\perp}}}\nonumber\\
    & \lep{a} \frac{N}{\alpha^{(\epsilon)}} { \left(\ex{\norm{\overline{\UU}}^{r'}_{r'} } \right)^{\frac{1}{r'}}  \left(\ex{\norm{\overline{\Q}^+_{\perp}}^r_r} \right)^{\frac{1}{r}}}.\nonumber\\
    & \lep{b} \frac{N}{\alpha^{(\epsilon)}}  \left(c_{r'} \epsilon \right)^{\frac{1}{r'}} \left(\ex{\norm{\overline{\Q}^+_{\perp}}^r_2} \right)^{\frac{1}{r}}.\nonumber\\
    & \lep{c}\frac{N}{\alpha^{(\epsilon)}}  \left(c_{r'} \epsilon \right)^{\frac{1}{r'}} \left(\ex{\norm{\overline{\Q}_{\perp}}^r_2} \right)^{\frac{1}{r}}.
  \end{align}
  where (a) follows from H\"older inequality for random vectors, and $r, r'\in (1,\infty)$ satisfy $1/r + 1/r' = 1$; (b) comes from Lemma \ref{lem:unused_service} and the fact that if $0<r_1 < r_2$, then $\norm{\mathbf{x}}_{r_2} \le \norm{\mathbf{x}}_{r_1}$ holds for any vector $\mathbf{x}$; (c) is true since the distribution of $\Q(t+1)$ and $\Q(t)$ are the same in steady-state.

  Thus, in order to prove the result in Proposition \ref{prop:prop_3}, we are left to characterize the moment of $\overline{\Q}_{\perp}$ in terms of the parameter $\delta^{(\epsilon)}$. First, combining Eq. \eqref{eq:drift_in_delta} and Claim \ref{claim_3}, yields
  \begin{equation*}
    \begin{split}
      &\ex{\Delta V_\perp(\Q) \mid \Q(t) = \Q }\\
       \le & \frac{1}{2\norm{\Qc(t)}} \ex{\left(2\inner{\Qc(t)}{\A(t) - \s(t)} + L\right) \mid \Q(t) = \Q}\\
       \le & -\frac{\mu_{\Sigma}\delta}{4N}  + \frac{L}{2\norm{\Qc(t)}}\\
       \le & -\frac{\mu_{\Sigma}\delta}{8N} \text{ for all } \Q \text{ such that } \norm{\Qc} \ge \frac{4NL}{\mu_{\Sigma}\delta}.
    \end{split}
  \end{equation*}
  Thus the condition (C1) in Lemma \ref{lem:basis} is valid with $\eta = \frac{\mu_{\Sigma}\delta}{8N}$ and $\kappa = \frac{4NL}{\mu_{\Sigma}\delta}$. Also, from Eq. \eqref{eq:boundedQc}, we have the condition (C2) is valid with $D = \sqrt{N} \max(A_{\max},S_{\max})$. Then from Eq. \eqref{eq:upper_siva} in Lemma \ref{lem:basis}, we get for $r = 1,2,\ldots,$
    \begin{align}
    \label{eq:moment_in_delta}
            \ex{\norm{\overline{\Q}_{\perp}}^r_2} &\le (2\kappa)^r + (4D)^r\left(\frac{D+\eta}{\eta} \right)^r r!\nonumber\\
            &\le \frac{1}{\delta^r}K_r^r
    \end{align}
    where $K_r \triangleq \left[ \left(\frac{8NL}{\mu_{\Sigma}}\right)^r + r! \left(\frac{32D^2N + 4D\mu_{\Sigma}}{\mu_{\Sigma}}\right)^r \right]^{\frac{1}{r}}$, which is independent of $\epsilon$. Now, substituting Eq. \eqref{eq:moment_in_delta} into Eq. \eqref{eq:upper_T_general}, yields
    \begin{align*}
      \mathcal{T}^{(\epsilon)} \le F_r\frac{\epsilon^{(1-1/r)}}{\alpha^{(\epsilon)}\delta^{(\epsilon)}}
    \end{align*}
    where $F_r \triangleq NK_r(S_{\max})^{(1/r^2 - 1/r)}$, which is independent of $\epsilon$. Since $\alpha^{(\epsilon)}\delta^{(\epsilon)} = \Omega(\epsilon^{\beta})$ and $\beta \in [0,1)$, there exists a positive $\beta'$ such that 
    \begin{align*}
      \mathcal{T}^{(\epsilon)} = O(\epsilon^{\beta'}),
    \end{align*}
    when $r > 1/(1-\beta)$. This directly implies that $\lim_{\epsilon \to 0}\mathcal{T}^{(\epsilon)} = 0$. Thus from Lemma \ref{claim_1}, the given policy is heavy-traffic delay optimal.
\end{proof}
